# Supplementary material for: Decentralized Role Assignment in Multi-Agent Teams via Empirical Game-Theoretic Analysis
Source: arXiv:2109.14755 source file (2021-09-29)
Supplement: Supplementary file 1 [file appendix.tex]

\appendix
\subsection{Collaborative Transport Environment}
\subsubsection{Environment}
The dynamics of the robots are modeled as a rigid rod, where the agents assert forces on the two ends of the rod to control the positional and angular acceleration of the bar. Specifically, denote the position of the two agents as $\vec{x^{(1)}} = (x^{(1)}, y^{(1)})$ and $\vec{x^{(2)}} = (x^{(2)}, y^{(2)})$, and denote the position of the midpoint of the bar as $x_{b}$ and the angle of the bar as $\alpha_{b}$. The agents have control over their force in both the x- and y-directions. Denote the control of agent i as $\vec{u}^{(i)}=(u^{(i)}_{x}, u^{(i)}_{y})$. Movement of the bar is then modeled as following
\begin{align*}
\ddot{x}_b &= \sum_{i} u^{(i)}\\
\ddot{\alpha}_i &= \sum_{i} u^{(i)} \times (\vec{x}^i-\vec{x}_b)\\
\end{align*}

The human agents in the environment are modeled as double integrators. Their control inputs follow a potential-field approach, where they are pushed away from the robotic agents and pulled by their respective destinations. Denote the human agent's position as $x^h$ and its destination as $x^{gh}$, its control at any point is given as \negar{what is humans' control input?}
\begin{align*}
 \frac{x^{gh} - x^h}{ ||x^h - x^{gh}||^2 } + \sum_{i=1}^2 \frac{x^h - x^{(i)}}{ ||x^h - x^{(i)}||^2 }
\end{align*}
Note that the human agents are not controllable and does not engage in game-theoretic control. We limit our planning considerations to the robots.

We clip the component-wise velocity and angular velocity of the bar and the agents to make the environment more realistic.

The robots start at $x^{(1)}_0 = (10,10)$, $x^{(2)}_0 = (30,10)$ and wants to move to $x^{g1} = (70,80)$, $x^{g2} = (90,80)$. The human agents start at $(10,10), (30,10)$ and want to move to $(20,80), (90,50)$, respectively. The velocities are capped elementwise at $1$ for the midpoint of the bar and for the agents. The angular velocity of the bar is capped at $0.05$ radians per step.

\subsubsection{Roles}
The controller for the leader is a sum of three components.
$$u_{leader} = (1-w) u^{g} + w u^{o} + u^{ca}$$
where $u^g, u^o, u^ca$ are respectively the positional, orientation, and collision avoidance controls. The positional control is in the direction of the goal position. The orientation control trys to adjust the angle of the rod to be horizontal. The collision avoidance control is found by a potential field approach and pushes the robot away from the human agents. $w$ is a weight parameter that controls the weight between orientation and positional control and goes to one as the agent gets closer to the goal position. Specifically, denote the goal of the agent as $x^{gl}$, then $w = \text{min}{1, \frac{1}{ ||x^{(i)} - x^{gl}|| }}$.

The control for the follower agent is given as follows,
$$u_{follower} = w \beta u_{leader} + (1-w) u^{o} + u^{ca}$$
where $u^o$ and $u^{ca}$ are found the same way as the leader. $ 0 < \beta < 1$ is a multiplier that specifies to what extent is the follower copying the leader's control. One thing to note here is that in reality the follower cannot always observe the leader's control in the same time step, so we have the follower copy the control of the leader in the previous time step.

\subsubsection{Payoff Structure}
Now the only thing waiting to be specified are the preferences of the agents. As mentioned before, the preferences of the agents come in three parts. First, they want to arrive to the destination as soon as possible. Secondly, they want to avoid collision with humans as much as possible. Thirdly, they want to expend as little control effort as possible. To capture this, we write down the running cost function for the agents as
$$g^i (x^{(1:2)}, u^{(1:2)}) = p_1 + p_2 \frac{1}{d_h} + p_3 ||u^{(i)}||$$
where $d_h$ is the minimal distance from any point on the rod to any human agent. $p_i$ controls the weighting between different types of costs. In the experiments, we have $p=(2,50,1.5)$.

\negar{you can cut some of the details in this section such as the specifics of the potential field to free up some space for more discussion of the algorithm and framework}

\negar{i remember that in your previous report, you had a subsection on solving empirical games, please try to include similar content in here too }
